# Supplementary material for: Self-assembly of colloidal polymers via depletion-mediated lock and key binding
Source: arXiv:1304.3675 source file (2014-01-10)
Supplement: Supplementary file 1 [file supplementary-v3-rev.pdf]

# Supplementary Information for "Self-assembly of colloidal polymers via depletion-mediated lock and key binding"

Douglas J. Ashton, Robert L. Jack and Nigel B. Wilding

This supplementary information provides full definitions of the quantities use in our calculations using Wertheim's theory (Sec. 4 of the main paper), and we explain how we calculate these quantities numerically.

### Definitions and numerical evaluation of $f_\mathrm{A}$, $K_0$, $v_1$, $v_2$.

In this section we will define the various quantities that go into the TPT and the self consistent Wertheim theory (SCW). Consider two anisotropic particles at positions $\boldsymbol{r}_1$, $\boldsymbol{r}_2$ with orientations $\boldsymbol{\omega}_1$, $\boldsymbol{\omega}_2$. The bond indicator function, $b(\boldsymbol{r}_1, \boldsymbol{r}_2, \boldsymbol{\omega}_1, \boldsymbol{\omega}_2)$, is defined such that $b = 1$ if particle 2 is bound within the lock site of particle 1, and $b = 0$ otherwise. For indented spheres, $b = 1$ if and only if the following three conditions are met: the two particles are not overlapping, the particle separation is less than $r_\mathrm{cut}$, and $\boldsymbol{n}_1 \cdot (\boldsymbol{r}_2 - \boldsymbol{r}_1) > \boldsymbol{n}_2 \cdot (\boldsymbol{r}_2 - \boldsymbol{r}_1)$, where $\boldsymbol{n}_1$, $\boldsymbol{n}_2$ are unit vectors pointing out through the centres of the indentations of particles 1 and 2. We always take $r_\mathrm{cut} < \sigma_l$, with $r_\mathrm{cut}$ being large enough to enclose the first peak in the radial distribution function, $g^\eta(r)$. (For the $AB$-patchy sphere model described in the main paper, $b = 1$ only when the $B$-patch of particle 2 is within a distance $\sigma_{AB}$ of the $A$-patch of particle 1.)

For the system with two indented spheres in a box of size $L$ and depletant at volume fraction $\eta$, let $P_L^\eta(\boldsymbol{r}_1, \boldsymbol{r}_2, \boldsymbol{\omega}_1, \boldsymbol{\omega}_2)$ be the probability that the two particles are found with these positions and orientations. Let

$$\tilde{g}_L^\eta(\boldsymbol{r}_1, \boldsymbol{r}_2, \boldsymbol{\omega}_1, \boldsymbol{\omega}_2) = P_L^\eta(\boldsymbol{r}_1, \boldsymbol{r}_2, \boldsymbol{\omega}_1, \boldsymbol{\omega}_2) \cdot \Omega^2 L^6,$$

where $\Omega$ is the phase space volume associated with the angular degrees of freedom (here $4\pi$). The tilde indicates that this distribution function is calculated from a system with just two indented colloids, so many-body effects are neglected. Let

$$\tilde{g}^\eta(\boldsymbol{r}_1, \boldsymbol{r}_2, \boldsymbol{\omega}_1, \boldsymbol{\omega}_2) = \lim_{L\to\infty} \tilde{g}_L^\eta(\boldsymbol{r}_1, \boldsymbol{r}_2, \boldsymbol{\omega}_1, \boldsymbol{\omega}_2).$$

The function $\tilde{g}^\eta$ contains all information about the effective pair potential between lock particles (in fact $\tilde{g}^\eta = \mathrm{e}^{-U/T}$ where $U$ is the effective pair potential and $T$ the temperature).

*Definition and numerical calculation of $f_\mathrm{A}$*

The definition of the Mayer function in equation (1) of the main text is

$$f_\mathrm{A}(\boldsymbol{r}_{12}, \boldsymbol{\omega}_1, \boldsymbol{\omega}_2) = b(\boldsymbol{r}_1, \boldsymbol{r}_2, \boldsymbol{\omega}_1, \boldsymbol{\omega}_2)[\tilde{g}^\eta(\boldsymbol{r}_1, \boldsymbol{r}_2, \boldsymbol{\omega}_1, \boldsymbol{\omega}_2) - 1],$$

where the right hand side depends on the particle positions only through $\boldsymbol{r}_{12} = \boldsymbol{r}_2 - \boldsymbol{r}_1$, by translational invariance.

When estimating the right hand side of equation (1) from simulation data, we replace $f_\mathrm{A}$ by an orientationally-averaged quantity $\overline{f_\mathrm{A}}(r) = \frac{1}{2}\Theta(r_\mathrm{cut} - r)[\frac{\tilde{g}^\eta(r)}{\tilde{g}^0(r)} - 1]$ (the factor of 2 arises because $\tilde{g}(r)$ receives contributions both when particle 2 is in the lock site of particle 1 and when particle 1 is in the lock site of particle 2, while the indicator function $b = 1$ only in the first case). Here, $\Theta(x)$ is the step function, and $\tilde{g}^\eta(r) = \frac{1}{\Omega^2}\int \mathrm{d}\boldsymbol{\omega}_1 \mathrm{d}\boldsymbol{\omega}_2 \tilde{g}(\boldsymbol{r}, \boldsymbol{\omega}_1, \boldsymbol{\omega}_2)$ is the radial distribution function between two indented colloids, with a similar expression for $\tilde{g}^0(r)$, the radial distribution function in the absence of depletant. Using this approximation when evaluating (1) greatly reduces the numerical complexity of the problem, without significant effects on our results.

*Definition and numerical calculation of $K_0$*

The definition of the bare equilibrium constant is $K_0 = \int \mathrm{d}\boldsymbol{r}_2 \frac{\mathrm{d}\boldsymbol{\omega}_1 \mathrm{d}\boldsymbol{\omega}_2}{\Omega^2} \tilde{g}^\eta(\boldsymbol{r}_1, \boldsymbol{r}_2, \boldsymbol{\omega}_1, \boldsymbol{\omega}_2) b(\boldsymbol{r}_1, \boldsymbol{r}_2, \boldsymbol{\omega}, \boldsymbol{\omega}')$. For numerical purposes, this can be obtained directly from the radial distribution function as

$$K_0 = \frac{1}{2}\int_0^{r_\mathrm{cut}} 4\pi r^2 \tilde{g}^\eta(r)\mathrm{d}r\,.$$

As in $\overline{f_\mathrm{A}}(r)$, the factor of 2 arises because $\tilde{g}(r)$ receives contributions both when particle 2 is in the lock site of particle 1 and when particle 1 is in the lock site of particle 2.

*Geometrical factors*

We now define various excluded volume factors that are arise when characterizing packing of indented spheres. For compactness, we use the notation $\boldsymbol{x} = (\boldsymbol{r}, \boldsymbol{\omega})$ and $\mathrm{d}\boldsymbol{x} = \mathrm{d}\boldsymbol{r}\mathrm{d}\boldsymbol{\omega}$.

*Definition of* $v_{\mathrm{MM}}$

The partition function for two free monomers (without depletant) in a single simulation box is

$$Z_{1,1} = \frac{1}{2}\int \mathrm{d}\boldsymbol{x}_1 \mathrm{d}\boldsymbol{x}_2 \cdot [1 + f_{\mathrm{R}}(\boldsymbol{x}_1, \boldsymbol{x}_2)] \tag{1}$$

where $f_{\mathrm{R}}(\boldsymbol{x}_i, \boldsymbol{x}_j) = -1$ if particles $i$ and $j$ are either overlapping or bonded, $f_{\mathrm{R}} = 0$ otherwise. The excluded volume between two particles is $v_{\mathrm{MM}}$ and may be obtained from $Z_{1,1} = \frac{1}{2}\Omega V \cdot \Omega(V - v_{\mathrm{MM}})$ where $V = L^3$ is the volume of the system. Further, the large-$r$ limit of the radial distribution function $\tilde{g}_L^0(r)$ is $\frac{1}{2}(V\Omega)^2/Z_{1,1}$ allowing $v_{\mathrm{MM}}$ to be evaluated numerically from $\tilde{g}_L^0(r)$.

*Definition of* $v_1$

The partition function for a bound dimer and a free monomer within a single box is

$$Z_{2,1} = \int \mathrm{d}\boldsymbol{x}_1 \mathrm{d}\boldsymbol{x}_2 \mathrm{d}\boldsymbol{x}_3\, \tilde{g}^{\eta}(\boldsymbol{x}_1, \boldsymbol{x}_2) b(\boldsymbol{x}_1, \boldsymbol{x}_2) \cdot [1 + f_{\mathrm{R}}(\boldsymbol{x}_1, \boldsymbol{x}_3)] \cdot [1 + f_{\mathrm{R}}(\boldsymbol{x}_2, \boldsymbol{x}_3)] \tag{2}$$

The definition of $v_1$ is such that $Z_{2,1} = (V\Omega) \cdot (K_0\Omega) \cdot (V - 2v_{\mathrm{MM}} + v_1)\Omega$. For numerical purposes, we simulate a monomer in a simulation box, together with a dimer made of two indented spheres bound by a patch interaction; we do not allow the particles to unbind during the simulation. We have used interactions that allow for different levels of flexibility within the dimer and find that this does not make any appreciable difference to the measured $v_1$. From this simulation we calculate the excluded volume between a monomer and a dimer, $v_{\mathrm{MD}}$, exactly as we do for $v_{\mathrm{MM}}$. Hence we can calculate $v_1 = 2v_{\mathrm{MM}} - v_{\mathrm{MD}}$.

*Definition of* $v_2$

The partition function for two dimers within a single box is

$$\begin{aligned} Z_{2,2} = \tfrac{1}{2} \int & \mathrm{d}\boldsymbol{x}_1 \mathrm{d}\boldsymbol{x}_2 \mathrm{d}\boldsymbol{x}_3 \mathrm{d}\boldsymbol{x}_4\, \tilde{g}^{\eta}(\boldsymbol{x}_1, \boldsymbol{x}_2) b(\boldsymbol{x}_1, \boldsymbol{x}_2) \cdot \tilde{g}^{\eta}(\boldsymbol{x}_3, \boldsymbol{x}_4) b(\boldsymbol{x}_3, \boldsymbol{x}_4) \\ & \times [1 + f_{\mathrm{R}}(\boldsymbol{x}_1, \boldsymbol{x}_3)] \cdot [1 + f_{\mathrm{R}}(\boldsymbol{x}_2, \boldsymbol{x}_3)] \cdot [1 + f_{\mathrm{R}}(\boldsymbol{x}_1, \boldsymbol{x}_4)] \cdot [1 + f_{\mathrm{R}}(\boldsymbol{x}_2, \boldsymbol{x}_4)] \end{aligned} \tag{3}$$

The definition of $v_2$ is such that $Z_{2,2} = \frac{1}{2}(K_0\Omega)^2 \cdot (V\Omega) \cdot (V - 4v_{\mathrm{MM}} + 4v_1 + v_2)\Omega$. For numerical purposes, we simulate two dimers, again comprised of two indented spheres held together with patches. The excluded volume between the dimers is $v_{\mathrm{DD}}$, from which we can obtain $v_2 = -4v_{\mathrm{MM}} + 4v_{\mathrm{MD}} - v_{\mathrm{DD}}$.
